# Supplementary material for: Instantaneous Quasiphoton in Strong-Field Ionization
Source: arXiv:2307.07220 source file (2024-02-15)
Supplement: Supplementary file 1 [file SuppMat.pdf]

# Quasiphoton at the Subcycle Level in Strong-Field Ionization

## —— Supplemental Material ——

Yongzhe Ma,<sup>1</sup> Hongcheng Ni,<sup>1,3</sup> Yang Li,<sup>2</sup> Feng He,<sup>2,4</sup> and Jian Wu<sup>1,3,4</sup>

<sup>1</sup>*State Key Laboratory of Precision Spectroscopy, East China Normal University, Shanghai 200241, China*

<sup>2</sup>*Key Laboratory for Laser Plasmas (Ministry of Education) and School of Physics and Astronomy,  
Collaborative Innovation Center for IFSA (CICIFSA), Shanghai Jiao Tong University, Shanghai 200240, China*

<sup>3</sup>*Collaborative Innovation Center of Extreme Optics, Shanxi University, Taiyuan, Shanxi 030006, China*

<sup>4</sup>*CAS Center for Excellence in Ultra-intense Laser Science, Shanghai 201800, China*

### S1. STRONG-FIELD APPROXIMATION

The concept of quasiphotons arises from the infinite-order dynamical symmetry present in the interaction between atoms and circularly or elliptically polarized light pulses. These quasiphotons can be characterized using a correlated spectrum of angular momentum and energy (SAME) of photoelectrons produced from strong-field ionization. The SAME in the asymptotic region can be obtained directly from the solutions of the time-dependent Schrödinger equation (TDSE) and the SAME at the tunnel exit can be extracted using the backpropagation method [1–4]. However, these methods fall short of a clear physical picture. To gain deeper insights into the fundamental light-matter interactions, we employ the strong-field approximation (SFA) [5, 6], which is capable of providing closed analytical expressions for the variables of interest. To this end, the transition amplitude between an atomic bound state and the continuum state with photoelectron asymptotic momentum  $\mathbf{p}$  is written as

$$M_{\mathbf{p}} = -i \int_{-\infty}^{+\infty} \langle \psi_{\mathbf{p}} | \mathbf{r} \cdot \mathbf{F}(t) | \psi_i \rangle dt, \quad (\text{S1})$$

where  $\mathbf{r}$  is the position operator,  $\mathbf{F}(t)$  is the electric field of the laser pulse,  $\psi_i(\mathbf{r}, t) = \psi_0(\mathbf{r})e^{iI_p t}$  is the bound-state wave function unperturbed by the laser field with  $I_p$  the ionization potential, and

$$\psi_{\mathbf{p}}(\mathbf{r}, t) = \exp \left\{ i[\mathbf{p} + \mathbf{A}(t)] \cdot \mathbf{r} - \frac{i}{2} \int^t [\mathbf{p} + \mathbf{A}(t')]^2 dt' \right\} \quad (\text{S2})$$

is the Volkov state (in the length gauge), where  $\mathbf{A}(t)$  is the vector potential of the laser pulse. With a further saddle-point approximation [7, 8], tunneling exit characteristics can be extracted within the SFA framework. Here, the saddle-point equation (SPE) reads

$$\frac{1}{2}[\mathbf{p} + \mathbf{A}(t_s)]^2 + I_p = 0, \quad (\text{S3})$$

where  $t_s = t_r + it_i$  is a complex solution to the SPE, with  $t_r$  the tunneling exit time and  $t_i$  relating to the ionization probability.

In the scenario of strong-field ionization, where the Keldysh parameter  $\gamma \approx \omega t_i$  is small, we may expand the vector potential  $\mathbf{A}(t_s)$  in terms of small  $t_i$  up to second order [3, 9–13]

$$\mathbf{A}(t_r + it_i) = \mathbf{A}(t_r) - it_i \mathbf{F}(t_r) + \frac{1}{2} t_i^2 \dot{\mathbf{F}}(t_r) + O(t_i^3), \quad (\text{S4})$$

where  $\dot{\mathbf{F}}(t_r) = \frac{d\mathbf{F}(t_r)}{dt_r}$ . Insertion of the expansion into the SPE [Eq. (S3)] results in

$$\mathbf{k}_{\perp}(t_r) \cdot \mathbf{F}(t_r) = 0, \quad (\text{S5})$$

$$t_i = \sqrt{\frac{k_{\perp}^2(t_r) + 2I_p}{F^2(t_r) - \mathbf{k}_{\perp}(t_r) \cdot \dot{\mathbf{F}}(t_r)}}, \quad (\text{S6})$$

where  $\mathbf{k}_{\perp}(t_r) = \mathbf{p}_{\perp} + \mathbf{A}(t_r)$  is the transverse momentum at the tunnel exit with the  $\perp$  subscript denoting variables in the polarization plane. The tunneling exit position can be obtained by

$$\mathbf{r}_0 = \text{Re} \int_{t_s}^{t_r} [\mathbf{p} + \mathbf{A}(t)] dt = \text{Im} \int_0^{t_i} \mathbf{A}(t_r + it) dt = -\frac{\mathbf{F}}{2} \frac{k_{\perp}^2 + 2I_p}{F^2 - \mathbf{k}_{\perp} \cdot \dot{\mathbf{F}}}, \quad (\text{S7})$$

and the angular momentum at the tunnel exit is subsequently obtained by

$$\mathbf{L} = \mathbf{r}_0 \times \mathbf{k}_{\perp} = \frac{F \mathbf{k}_{\perp}}{2} \frac{k_{\perp}^2 + 2I_p}{F^2 - \mathbf{k}_{\perp} \cdot \dot{\mathbf{F}}} \mathbf{e}_z = \frac{k_{\perp}(k_{\perp}^2 + 2I_p)}{2(F + \tilde{\epsilon} \omega k_{\perp})} \mathbf{e}_z, \quad (\text{S8})$$

where a slowly varying envelope approximation has been applied in the last step and

$$\tilde{\varepsilon} = \frac{\varepsilon}{\varepsilon^2 \cos^2(\omega t) + \sin^2(\omega t)}. \quad (\text{S9})$$

The energy at the tunnel exit is

$$E = \frac{1}{2}k_{\perp}^2 + \mathbf{r}_0 \cdot \mathbf{F}(t) = \frac{1}{2}k_{\perp}^2 - \frac{F^2}{2} \frac{k_{\perp}^2 + 2I_p}{F^2 - \mathbf{k}_{\perp} \cdot \mathbf{F}} = \frac{\tilde{\varepsilon} \omega k_{\perp}^3 - 2I_p F}{2(F + \tilde{\varepsilon} \omega k_{\perp})} = \tilde{\varepsilon} \omega \frac{k_{\perp}(k_{\perp}^2 + 2I_p)}{2(F + \tilde{\varepsilon} \omega k_{\perp})} - I_p = \tilde{\varepsilon} \omega L_z - I_p. \quad (\text{S10})$$

Clearly, for the elliptical polarization, the quasiphoton has different angular frequencies or energies throughout the optical cycle, ranging from  $\varepsilon \omega$  to  $\omega/\varepsilon$ . For circular polarization where  $\varepsilon = 1$ , we have  $\tilde{\varepsilon} = 1$ , the above relation reduces to

$$E = \omega L_z - I_p, \quad (\text{S11})$$

where the quasiphoton has a fixed angular frequency of  $\omega$ , in coincident to the photon energy.

To assess the behavior of quasiphotons at the subcycle level, we show the SAME at the tunnel exit at different time instances, see Figs. S1 and S2 corresponding to circular and elliptical light pulses, respectively. In the case of circular pulse as shown in Fig. S1, the SAME consistently adheres to the same circular conservation law [Eq. (S11)] at all time instances, even in the presence of pulse envelope. This indicates the existence of quasiphotons at the subcycle level. Interestingly, the quasiphotons possess an energy that is identical to the normal photons. For elliptical pulse as shown in Fig. S2, the SAME follows straight lines as well, albeit with varying slope at different time instances. Close scrutiny reveals that the slope varies between  $\varepsilon \omega$  and  $\omega/\varepsilon$ , in agreement with the above theoretical formulations. When the electric field peaks, the slope is  $\varepsilon \omega$ ; while when the electric field reaches minima, the slope becomes  $\omega/\varepsilon$ . This points to the fact that quasiphotons have different effective angular frequencies or energies at different time instances within an optical cycle. Since tunneling ionization is a highly nonlinear process, the ionization rate is exponentially related to the electric field strength, the time-integrated SAME thus has roughly a slope of  $\varepsilon \omega$ .

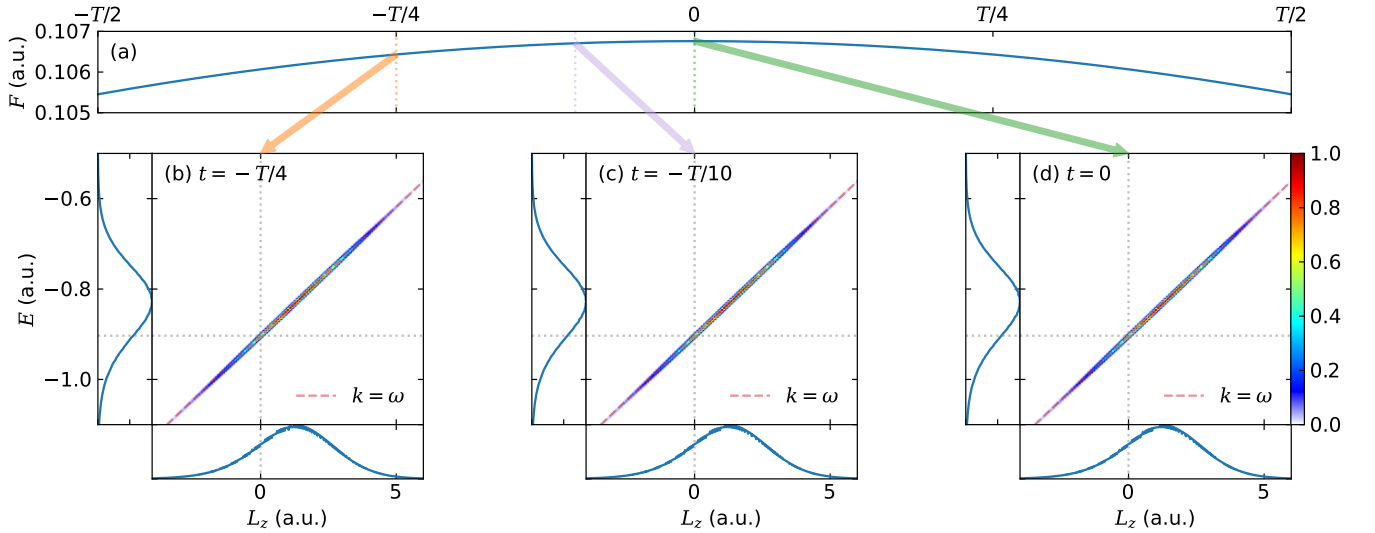

FIG. S1. (a) Total electric field magnitude  $F$  of a circularly polarized laser pulse. (b-d) Correlation spectrum of angular momentum and energy (SAME) of photoelectrons at the tunnel exit ionized at different time instances. In panels (b-d), the left subfigure shows the distribution of energy, and the lower subfigure shows the distribution of angular momentum. The red dashed line denotes  $E = \omega L_z - I_p$ . Note that the color maps are normalized across different time instances.

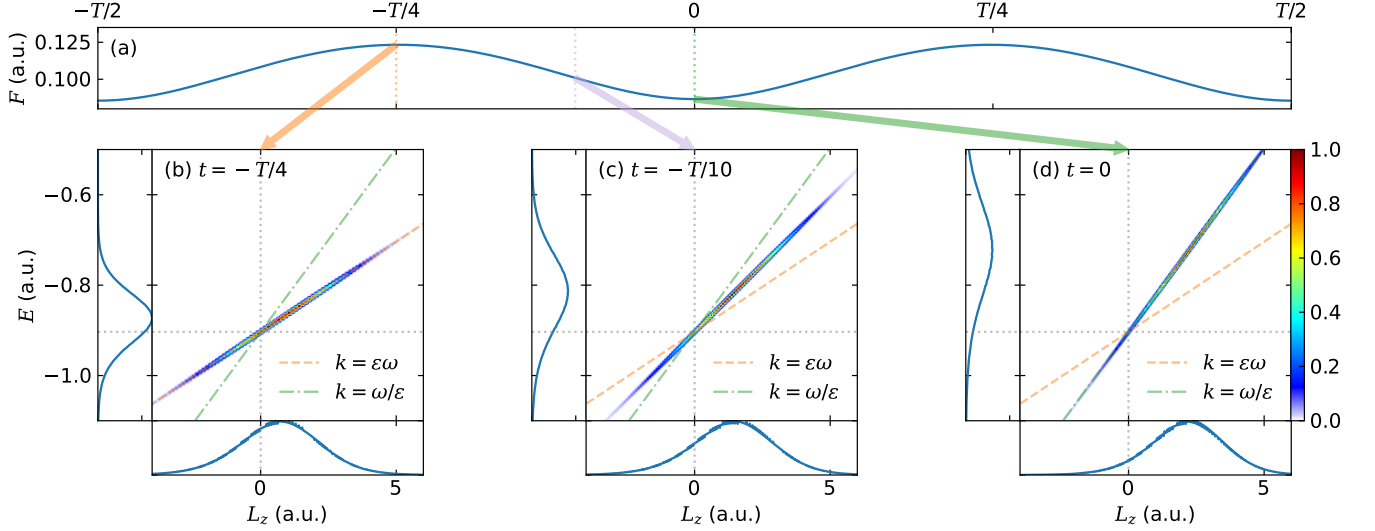

FIG. S2. (a) Total electric field magnitude  $F$  of an elliptically polarized laser pulse with ellipticity  $\varepsilon = 0.7$ . (b-d) Correlation spectrum of angular momentum and energy (SAME) of photoelectrons at the tunnel exit ionized at different time instances. In panels (b-d), the left subfigure shows the distribution of energy, and the lower subfigure shows the distribution of angular momentum. The orange dashed line denotes  $E = \varepsilon\omega L_z - I_p$  and the green dash-dotted line denotes  $E = (\omega/\varepsilon)L_z - I_p$ . Note that the color maps are normalized across different time instances.

## S2. PHASE RETRIEVAL AND QUASIPHOTON IN THE ASYMPTOTIC REGION

To uncover the behavior of quasiphotons in the asymptotic region, we need to construct the SAME from the asymptotic photoelectron momentum distribution. While energy is easily obtained from the momentum distribution, the evaluation of angular momentum is nontrivial since its information is encoded in the phase structure of the photoelectron momentum distribution. To retrieve the phase information, one would naturally consider to design an approach which brings together two exact replicas of the same original pattern where the phase information can be decoded from the interference pattern originating from the two replicas. This is exactly what we do here in this study. We employ two time-delayed counter-rotating circularly polarized light pulses to induce interferences in the photoelectron momentum distribution known as electron vortices [14–17], with the total field defined by

$$\mathbf{A}(t) = A_0 \cos^4\left(\frac{\omega t}{2N}\right) \begin{pmatrix} \cos(\omega t) \\ \sin(\omega t) \end{pmatrix} + A_0 \cos^4\left[\frac{\omega(t-\tau)}{2N}\right] \begin{pmatrix} \cos[\omega(t-\tau)] \\ -\sin[\omega(t-\tau)] \end{pmatrix}, \quad (\text{S12})$$

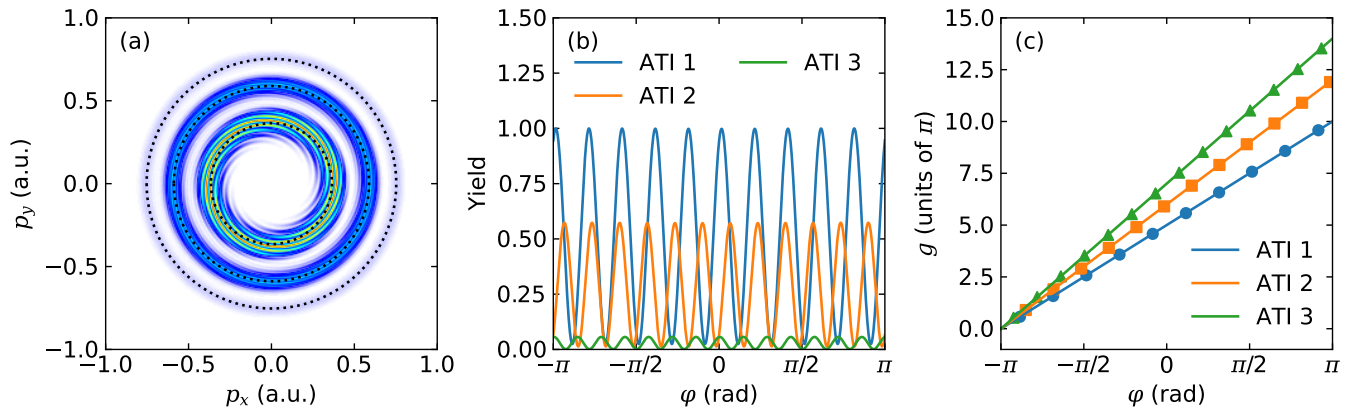

FIG. S3. (a) Photoelectron momentum distribution resulting from the ionization of hydrogen atoms by the time-delayed counter-rotating circularly polarized laser pulse after focal volume averaging. (b) Yield at different ATI orders corresponding to the black dotted line in panel (a). (c) Phase  $g$  extracted from the vortex structure.

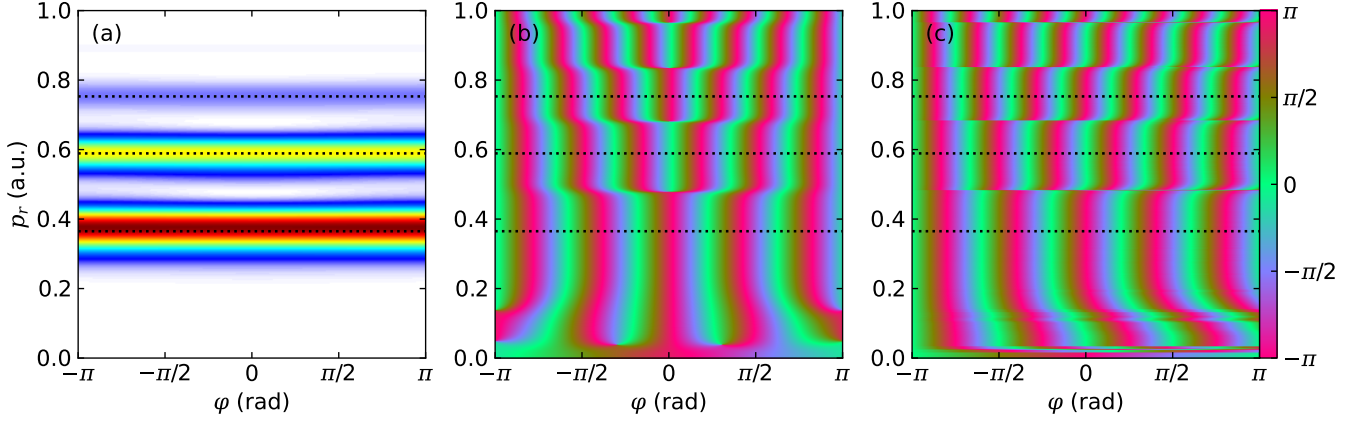

FIG. S4. (a) Momentum and (b) phase distribution of electron wave packets ionized by a circularly polarized laser pulse obtained by direct numerical evaluation of Eq. (S1). (c) Phase distribution extracted through the vortex structure. The distributions are shown in polar coordinate.

where  $\tau$  is the time delay between the two circular pulses.

Shown in Fig. S3(a) is the photoelectron momentum distribution obtained using SFA resulting from the ionization of hydrogen atoms by the time-delayed counter-rotating circularly polarized pulse, where clear electron vortex structures are visible. Each individual circular pulse has a wavelength of 400 nm and an optical cycle number  $N = 10$ . The peak-to-peak time delay between the two pulses is  $\tau = 11T$ . In addition, we have performed focal volume averaging, where a total of 15 different intensities are calculated in the range of  $I = 2.0 \sim 3.4 \times 10^{13}$  W/cm<sup>2</sup> and the results are summed with a weight given by  $(I_0 + 2I)\sqrt{I_0 - I}/I^{5/2}$  [18, 19], where  $I_0 = 3.4 \times 10^{13}$  W/cm<sup>2</sup> is the peak intensity.

To retrieve the phase information from the electron vortex structure, we write down the amplitude of ionization by one individual circular pulse as  $M_p \propto R(p)\exp(ig(\varphi))$ , where  $R(p)$  is a real function of the electron momentum and  $g(\varphi)$  stands for an angular phase distribution [20]. Thereby, the electron wave packet ionized by the two time-delayed counter-rotated circularly polarized laser pulses can be approximated as

$$\Psi = R(p)\exp(-iE_p\tau)\exp(ig(\varphi)) + R(p)\exp(iI_p\tau)\exp(-ig(\varphi)), \quad (\text{S13})$$

where  $E_p = p^2/2$ . The vortex structure can then be expressed as

$$|\Psi|^2 = 2R(p) \{1 + \cos[(E_p + I_p)\tau - 2g(\varphi)]\}. \quad (\text{S14})$$

Evidently, the angular distribution exhibits cosine oscillations at specific energies, see Fig. S3(b). At oscillation valleys, the phase  $g(\varphi)$  satisfies  $(E_p + I_p)\tau - 2g(\varphi) = (2n + 1)\pi$  with  $n \in \mathbb{Z}$ . Hence, the phase of the electronic wave packet can be extracted from the minima of the oscillations. An additional fit to the phase  $g(\varphi)$  leads to an well-defined expression of  $g(\varphi)$ , as shown in Fig. S3(c). Repeating the procedure for all energies, we can construct the momentum-resolved phase distribution, as shown in Fig. S4(c). In order to check the accuracy of the extracted phase, we directly calculate the momentum-resolved phase distribution by numerically evaluating Eq. (S1), and the resulting distribution is depicted in Fig. S4(b). Clearly, the retrieved phase distribution agrees well with direct numerical results, which means the present phase retrieval procedure is reliable. It is worth noting that the extracted phase is only accurate near the ATI peaks, as shown in Fig. S4(a), marked by the black dotted lines.

With the reliably retrieved phase distribution of the photoelectron momentum distribution, the angular momentum distribution in the asymptotic region can be obtained by applying the angular momentum operator  $\hat{L}_z = -i\frac{\partial}{\partial\varphi}$  to the complex amplitude of photoelectron wave packet in the momentum space. The SAME in the asymptotic region can be subsequently constructed, as shown in Fig. 4(b) of the main text. Remarkably, the conservation law in the asymptotic region follows slightly differently from that at the tunnel exit in the form of

$$E = \omega L_z - I_p - U_p, \quad (\text{S15})$$

with an additional ponderomotive term  $-U_p$ .

We proceed to investigate the behavior of quasiphotons at the subcycle level, i.e., at different emission angles in the asymptotic region, see Fig. S5. Evidently, the SAME adheres to the same conservation law at different emission angles, or at different time instances within an optical cycle.

We stress that, unlike previous studies [20, 21], where *ad hoc* assumptions regarding the phase  $g(\varphi)$  are made, our phase retrieval procedure is free from assumptions. Therefore, the present study provides unambiguous support for the definition of quasiphotons at the subcycle level, both at the tunnel exit and in the asymptotic region.

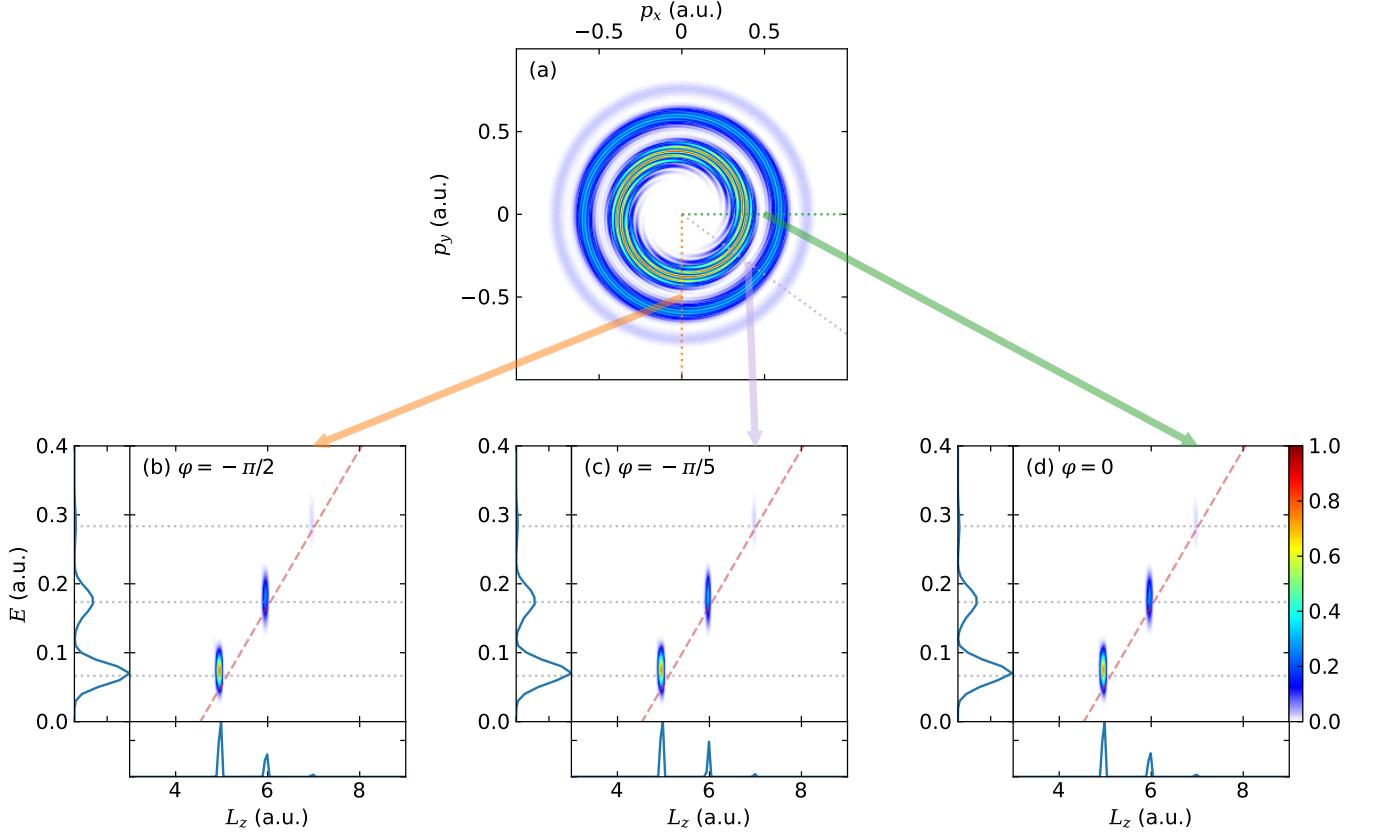

FIG. S5. (a) Photoelectron momentum distribution resulting from the ionization of hydrogen atoms by the time-delayed counter-rotating circularly polarized laser pulse after focal volume averaging. (b-d) Correlated spectrum of angular momentum and energy at different emission angles. The red dashed line denotes  $E = \omega L_z - I_p - U_p$ .

### S3. INFLUENCE OF COULOMB POTENTIAL

Comparing Figs. 2(a1) and 2(b1) of the main text, we find that the SAME in Fig. 2(b1), obtained from SFA, adheres closely to the conservation law [eq. (S11)], while that in Fig. 2(a1), obtained from backpropagation, has a slight downward offset and curvature with respect to the conservation law. Both effects are due to the influence of the Coulomb potential of the parent ion. To elucidate this point, we show in Fig. S6 a comparison of the SAME obtained from different methods, where Fig. S6(a) is obtained from backpropagation of the full helium single-active-electron potential [22]

$$V(r) = -\frac{Z_c + a_1 e^{-a_2 r} + a_3 r e^{-a_4 r} + a_5 e^{-a_6 r}}{r}, \quad (\text{S16})$$

where  $Z_c = 1.0$ ,  $a_1 = 1.231$ ,  $a_2 = 0.662$ ,  $a_3 = -1.325$ ,  $a_4 = 1.236$ ,  $a_5 = -0.231$ ,  $a_6 = 0.480$ ; Fig. S6(b) is obtained from backpropagation of a short-range potential of the form

$$V(r) = -\frac{e^{-100r} + e^{-r^2/2}}{\sqrt{r^2 + a}}, \quad (\text{S17})$$

where the soft-core parameter  $a$  is tuned so that the ionization potential matches that of the helium atom; and Fig. S6(c) is obtained from SFA which takes full account of the pulse envelope. Comparing Figs. S6(a) and S6(b), it is clear that the offset is smaller for the short-range potential. Needless to say, the short-range potential still differs from a zero-range potential as in the case of SFA. That is why the SAME in Fig. S6(b) still has a small offset, while that from SFA as in Fig. S6(c) has zero offset. In addition, the SAME obtained from SFA in Fig. S6(c) fully accounts for the pulse envelope, so the curvature in Figs. S6(a) and S6(b) also arises from the influence of the Coulomb potential.

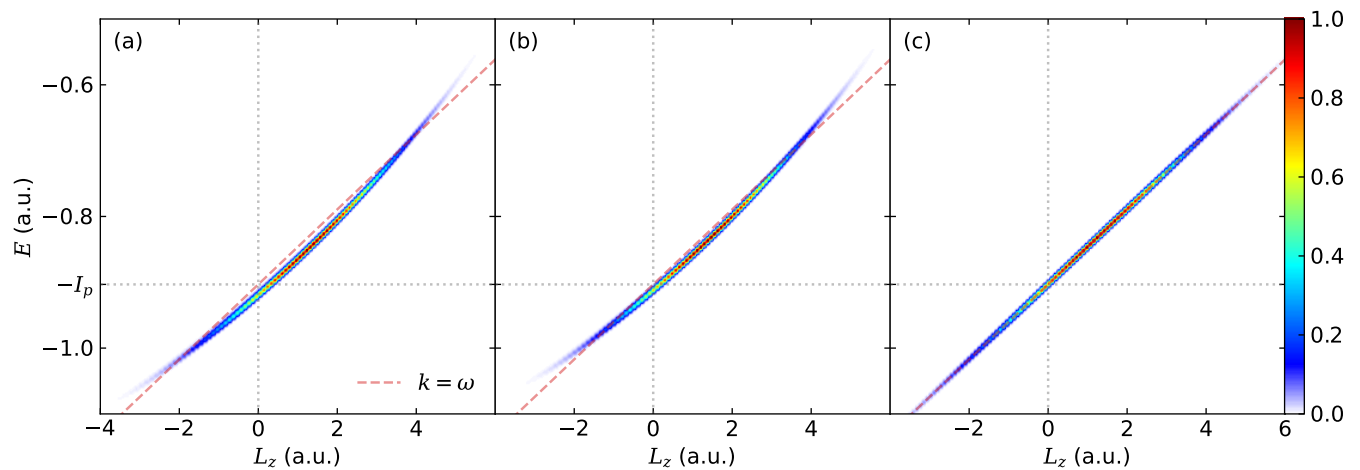

FIG. S6. Correlated spectrum of angular momentum and energy (SAME) of photoelectrons at the tunnel exit obtained from (a) backpropagation of the helium potential, (b) backpropagation of the short-range potential, and (c) SFA.

- 
- [1] H. Ni, U. Saalmann, and J.-M. Rost, Tunneling ionization time resolved by backpropagation, *Phys. Rev. Lett.* **117**, 023002 (2016).
  - [2] H. Ni, U. Saalmann, and J.-M. Rost, Tunneling exit characteristics from classical backpropagation of an ionized electron wave packet, *Phys. Rev. A* **97**, 013426 (2018).
  - [3] H. Ni, N. Eicke, C. Ruiz, J. Cai, F. Oppermann, N. I. Shvetsov-Shilovski, and L.-W. Pi, Tunneling criteria and a nonadiabatic term for strong-field ionization, *Phys. Rev. A* **98**, 013411 (2018).
  - [4] C. Hofmann, A. Bray, W. Koch, H. Ni, and N. I. Shvetsov-Shilovski, Quantum battles in attoscience: tunnelling, *Eur. Phys. J. D* **75**, 208 (2021).
  - [5] S. V. Popruzhenko, *J. Phys. B* **47**, 204001 (2014).
  - [6] K. Amini, J. Biegert, F. Calegari, A. Chacón, M. F. Ciappina, A. Dauphin, D. K. Efimov, C. Figueira de Morisson Faria, K. Giergiel, P. Gniewek, A. S. Landsman, M. Lesiuk, M. Mandrysz, A. S. Maxwell, R. Moszyński, L. Ortmann, J. Antonio Pérez-Hernández, A. Picón, E. Pisanty, J. Prauzner-Bechcicki, K. Sacha, N. Suárez, A. Zaïr, J. Zakrzewski, and M. Lewenstein, Symphony on strong field approximation, *Rep. Prog. Phys.* **82**, 116001 (2019).
  - [7] A. Nayak, M. Dumergue, S. Kühn, S. Mondal, T. Csizmadia, N. Harshitha, M. Füle, M. Upadhyay Kahaly, B. Farkas, B. Major, V. Szaszko-Bogár, P. Földi, S. Majorosi, N. Tsatrafyllis, E. Skantzakis, L. Neoričić, M. Shirozhan, G. Vampa, K. Varjú, P. Tzallas, G. Sansone, D. Charalambidis, and S. Kahaly, Saddle point approaches in strong field physics and generation of attosecond pulses, *Phys. Rep.* **833**, 1 (2019).
  - [8] A. Jašarević, E. Hasović, R. Kopold, W. Becker, and D. B. Milošević, Application of the saddle-point method to strong-laser-field ionization, *J. Phys. A* **53**, 125201 (2020).
  - [9] S. P. Goreslavski, G. G. Paulus, S. V. Popruzhenko, and N. I. Shvetsov-Shilovski, Coulomb asymmetry in above-threshold ionization, *Phys. Rev. Lett.* **93**, 233002 (2004).
  - [10] M. V. Frolov, N. L. Manakov, A. A. Minina, S. V. Popruzhenko, and A. F. Starace, Adiabatic-limit coulomb factors for photoelectron and high-order-harmonic spectra, *Phys. Rev. A* **96**, 023406 (2017).
  - [11] H. Ni, S. Brennecke, X. Gao, P.-L. He, S. Donsa, I. Březinová, F. He, J. Wu, M. Lein, X.-M. Tong, and J. Burgdörfer, Theory of subcycle linear momentum transfer in strong-field tunneling ionization, *Phys. Rev. Lett.* **125**, 073202 (2020).
  - [12] Y. Ma, J. Zhou, P. Lu, H. Ni, and J. Wu, Influence of nonadiabatic, nondipole and quantum effects on the attoclock signal, *J. Phys. B* **54**, 144001 (2021).
  - [13] X. Mao, H. Ni, X. Gong, J. Burgdörfer, and J. Wu, Subcycle-resolved strong-field tunneling ionization: Identification of magnetic dipole and electric quadrupole effects, *Phys. Rev. A* **106**, 063105 (2022).
  - [14] J. M. Ngoko Djiokap, S. X. Hu, L. B. Madsen, N. L. Manakov, A. V. Meremianin, and A. F. Starace, Electron vortices in photoionization by circularly polarized attosecond pulses, *Phys. Rev. Lett.* **115**, 113004 (2015).
  - [15] J. M. Ngoko Djiokap, A. V. Meremianin, N. L. Manakov, S. X. Hu, L. B. Madsen, and A. F. Starace, Multistart spiral electron vortices in ionization by circularly polarized uv pulses, *Phys. Rev. A* **94**, 013408 (2016).
  - [16] D. Pengel, S. Kerbstadt, D. Johannmeyer, L. Englert, T. Bayer, and M. Wollenhaupt, Electron vortices in femtosecond multiphoton ionization, *Phys. Rev. Lett.* **118**, 053003 (2017).
  - [17] D. Pengel, S. Kerbstadt, L. Englert, T. Bayer, and M. Wollenhaupt, Control of three-dimensional electron vortices from femtosecond multiphoton ionization, *Phys. Rev. A* **96**, 043426 (2017).
  - [18] S. Augst, D. D. Meyerhofer, D. Strickland, and S. L. Chin, Laser ionization of noble gases by coulomb-barrier suppression, *J. Opt. Soc. Am. B* **8**, 858 (1991).

- [19] M.-M. Liu, M. Li, C. Wu, Q. Gong, A. Staudte, and Y. Liu, Phase structure of strong-field tunneling wave packets from molecules, [Phys. Rev. Lett. \*\*116\*\*, 163004 \(2016\)](#).
- [20] X.-R. Xiao, M.-X. Wang, H. Liang, Q. Gong, and L.-Y. Peng, Proposal for measuring electron displacement induced by a short laser pulse, [Phys. Rev. Lett. \*\*122\*\*, 053201 \(2019\)](#).
- [21] Y.-N. Qin, M. Li, Y. Feng, S. Luo, Y. Zhou, and P. Lu, Extracting the phase distribution of the electron wave packet ionized by an elliptically polarized laser pulse, [Front. Phys. \*\*16\*\*, 1 \(2021\)](#).
- [22] X. M. Tong and C. D. Lin, Empirical formula for static field ionization rates of atoms and molecules by lasers in the barrier-suppression regime, [J. Phys. B \*\*38\*\*, 2593 \(2005\)](#).
